# Supplementary material for: HyP-ABC: A Novel Automated Hyper-Parameter Tuning Algorithm Using Evolutionary Optimization
Source: arXiv:2109.05319 source file (2021-09-11)
Supplement: Supplementary file 1 [file suplementary.tex]

\documentclass[conference]{IEEEtran}
\usepackage{cite}
\usepackage{amsmath,amssymb,amsfonts}
\usepackage{algorithmic}
\usepackage{graphicx}
\usepackage{dblfloatfix}
\usepackage{textcomp}
\usepackage{xcolor}
\usepackage{calc}
\usepackage{ifthen}
\usepackage{tikz,amsmath}
\usepackage{algorithmic}
\usepackage{algorithm}
\usepackage{comment}
\usepackage{eqparbox}
\usepackage{makecell}
\usepackage{adjustbox}
\usepackage[normalem]{ulem}

\usepackage{pgfplots}
\usepackage{tikz}
\usepackage{xcolor}
\usepackage[normalem]{ulem}
% Define bar chart colors
%
\definecolor{bblue}{HTML}{4F81BD}
\definecolor{rred}{HTML}{C0504D}
\definecolor{ggreen}{HTML}{9BBB59}
\definecolor{ppurple}{HTML}{9F4C7C}
\definecolor{yyellow}{HTML}{FFD700}
\definecolor{ppink}{HTML}{FE6F5E}
\definecolor{purpule}{HTML}{BF94E4}

%\usepackage{algorithmicx}
%\usepackage{algpseudocode}	
% algorithmic.sty was written by Peter Williams and Rogerio Brito.
% This package provides an algorithmic environment fo describing algorithms.
% You can use the algorithmic environment in-text or within a figure
% environment to provide for a floating algorithm. Do NOT use the algorithm
% floating environment provided by algorithm.sty (by the same authors) or
% algorithm2e.sty (by Christophe Fiorio) as the IEEE does not use dedicated
% algorithm float types and packages that provide these will not provide
% correct IEEE style captions. The latest version and documentation of
% algorithmic.sty can be obtained at:
% http://www.ctan.org/pkg/algorithms
% Also of interest may be the (relatively newer and more customizable)
% algorithmicx.sty package by Szasz Janos:
% http://www.ctan.org/pkg/algorithmicx

% *** ALIGNMENT PACKAGES ***
%
\usepackage{array}
\usepackage{fixltx2e}
\usepackage{dblfloatfix}
% The latest version can be found at:
% http://www.ctan.org/pkg/dblfloatfix

% *** PDF, URL AND HYPERLINK PACKAGES ***
%
%usepackage{url}
% url.sty was written by Donald Arseneau. It provides better support for
% handling and breaking URLs. url.sty is already installed on most LaTeX
% systems. The latest version and documentation can be obtained at:
% http://www.ctan.org/pkg/url
% Basically, \url{my_url_here}.

% *** Do not adjust lengths that control margins, column widths, etc. ***
% *** Do not use packages that alter fonts (such as pslatex).         ***
% There should be no need to do such things with IEEEtran.cls V1.6 and later.
% (Unless specifically asked to do so by the journal or conference you plan
% to submit to, of course. )

% correct bad hyphenation here
% \hyphenation{op-tical net-works semi-conduc-tor}

\begin{document}
%
% paper title
% Titles are generally capitalized except for words such as a, an, and, as,
% at, but, by, for, in, nor, of, on, or, the, to and up, which are usually
% not capitalized unless they are the first or last word of the title.
% Linebreaks \\ can be used within to get better formatting as desired.
% Do not put math or special symbols in the title.
\title{Supplementary Material}
% make the title area

% author names and affiliations
% use a multiple column layout for up to three different
% affiliations

% conference papers do not typically use \thanks and this command
% is locked out in conference mode. If really needed, such as for
% the acknowledgment of grants, issue a \IEEEoverridecommandlockouts
% after \documentclass

% for over three affiliations, or if they all won't fit within the width
% of the page, use this alternative format:
% 
%\author{\IEEEauthorblockN{Michael Shell\IEEEauthorrefmark{1},
%Homer Simpson\IEEEauthorrefmark{2},
%James Kirk\IEEEauthorrefmark{3}, 
%Montgomery Scott\IEEEauthorrefmark{3} and
%Eldon Tyrell\IEEEauthorrefmark{4}}
%\IEEEauthorblockA{\IEEEauthorrefmark{1}School of Electrical and Computer Engineering\\
%Georgia Institute of Technology,
%Atlanta, Georgia 30332--0250\\ Email: see http://www.michaelshell.org/contact.html}
%\IEEEauthorblockA{\IEEEauthorrefmark{2}Twentieth Century Fox, Springfield, USA\\
%Email: homer@thesimpsons.com}
%\IEEEauthorblockA{\IEEEauthorrefmark{3}Starfleet Academy, San Francisco, California 96678-2391\\
%Telephone: (800) 555--1212, Fax: (888) 555--1212}
%\IEEEauthorblockA{\IEEEauthorrefmark{4}Tyrell Inc., 123 Replicant Street, Los Angeles, California 90210--4321}}

% use for special paper notices
%\IEEEspecialpapernotice{(Invited Paper)}

\maketitle

% As a general rule, do not put math, special symbols or citations
% in the abstract
\section{Leveraged ML Algorithms}
A summary of the ML algorithms used in this study as follows:
\begin{enumerate}
    \item \textbf{Random Forest (RF)} \cite{breiman2001random} is an ensemble method and a type of Decision Tree (DT) learner that operates by constructing many DTs in the training phase. That is the reason it is called 'forest.' The term 'random' is also because the trees are built differently with random samples and random features to add diversity to the models and decrease the chance of overfitting \cite{breiman2001random,liaw2002classification,louppe2014understanding}. Random forest initially uses the bagging method to combine the predictions from each tree and calculate the overall predictions.

%========================================

    \item \textbf{eXtreme Gradient Boosting (XGBoost)} \cite{chen2015xgboost} is a developed version of Gradient Boosting that utilizes a gradient boosting framework as an ensemble. One of the XGBoost focuses is the efficiency and speed of the model and supports parallelization. Focusing on the computational speed and model efficiency. XGBoost also tries to prevent overfitting using Ridge and Lasso regularization. XGBoost trains the model iteratively, correcting or fixing the newer models in each iteration \cite{chen2017xgboost}. XGBoost also has internal cross-validation. Hence, there is no need to identify the number of iterations in each run.

    \item \textbf{Support Vector Machine (SVM)} is a supervised learning technique that generates input-output mapping functions. The mapping function in the purpose of this study is a classification function, in which nonlinear kernel functions are used to transform input to a high-dimensional feature space. In this feature space, the data become more separable when compared to the raw input. SVM works by finding the maximum-margin hyper-planes between positive and negative observations. Using mapping function, SVM transforms the non-separable feature to linearly separable features \cite{wang2005support,shalev2014understanding}.
\end{enumerate}

\section{Main Hyper-parameters}
Applying ML algorithms to different problems, only several hyper-parameters significantly impact the model's performance. These parameters are the main hyper-parameters of the model that require  tuning\cite{yang2020hyperparameter}. Although the rest of the hyper-parameters may have a slight impact on the performance but they also increase the search space scales. The increase in the number of hyper-parameters increases the number of configurations exponentially, and as a result, the tuning time also increases \cite{decastro2019effect}. Therefore we reduce the impact of large space on tuning time by only considering the main hyper-parameters of ML models. 
To put theory into practice, we conducted our experiment based on Table \ref{tab:MainHP} that provides a summary of the applied ML algorithms and their main hyper-parameters.

\begin{table}[ht]
\centering
\caption{ML Classifiers' Main Hyper-parameters}
\label{tab:MainHP}
%\begin{adjustbox}{width=\columnwidth,cente}
\def\arraystretch{1}
\begin{tabular}{|c|c|}
\hline
\textbf{ML Classifier} & \textbf{Main Hyper-parameters}\\
\hline
\textbf{RF}   &  \makecell{n\_estimators, criterion, max\_depth, max\_features,\\ min\_samples\_split, min\_samples\_leaf}  \\
\hline
\textbf{XGBoost} & \makecell{n\_estimators, max\_depth, learning\_rate,\\ subsample, colsample\_bytree}   \\
\hline
\textbf{SVM} &  \makecell{C, kernel}  \\
\hline
\end{tabular}
%\end{adjustbox}
\end{table}
\section{Search Spaces}
Table \ref{tab:search} shows the details of hyper-parameters' search space configured for this study as well as their ranges and type. The determined search scales are based on testings and domain knowledge. 

\begin{table}[ht]
\centering
\caption{ML Classifiers' Main Hyper-parameters}
\label{tab:search}
%\begin{adjustbox}{width=\columnwidth,cente}
\def\arraystretch{1.2}
\begin{tabular}{|c|c|c|}
\hline
\textbf{Hyper-parameter} & \textbf{Search Space} & \textbf{Type}\\
\hline
\textbf{n\_estimators}   &  \makecell{  [5,500] } & Integer \\
\hline
\textbf{criterion} & \makecell{ [gini, entropy]  } & Categorical \\
\hline
\textbf{max\_depth} &  \makecell{ [5,50]} & Integer \\
\hline
\textbf{max\_features} &  \makecell{ [1,91]} & Integer \\
\hline
\textbf{min\_samples\_split} &  \makecell{ [2,30]} & Integer\\
\hline
\textbf{min\_samples\_leaf} &  \makecell{[1,15]} & Integer \\
\hline
\textbf{learning\_rate} &  \makecell{ [0,1]} & Continuous\\
\hline
\textbf{subsample} &  \makecell{(0,1]} & Continuous\\
\hline
\textbf{colsample\_bytree} &  \makecell{(0,1]} & Continuous\\
\hline
\textbf{C} &  \makecell{ [0.1,50]} & Continuous\\
\hline
\textbf{Kernel} &  \makecell{linear, poly, rbf, sigmoid} & Categorical\\
\hline
\end{tabular}
%\end{adjustbox}
\end{table}

% use section* for acknowledgment
%\section*{Acknowledgment}

% trigger a \newpage just before the given reference
% number - used to balance the columns on the last page
% adjust value as needed - may need to be readjusted if
% the document is modified later
%\IEEEtriggeratref{8}
% The "triggered" command can be changed if desired:
%\IEEEtriggercmd{\enlargethispage{-5in}}

% references section

% can use a bibliography generated by BibTeX as a .bbl file
% BibTeX documentation can be easily obtained at:
% http://mirror.ctan.org/biblio/bibtex/contrib/doc/
% The IEEEtran BibTeX style support page is at:
% http://www.michaelshell.org/tex/ieeetran/bibtex/
%\bibliographystyle{IEEEtran}
% argument is your BibTeX string definitions and bibliography database(s)
%\bibliography{IEEEabrv,../bib/paper}
%
% <OR> manually copy in the resultant .bbl file
% set second argument of \begin to the number of references
% (used to reserve space for the reference number labels box)

% \begin{thebibliography}{1}
% \newpage
% \bibitem{IEEEhowto:kopka}
% H.~Kopka and P.~W. Daly, \emph{A Guide to \LaTeX}, 3rd~ed.\hskip 1em plus
%   0.5em minus 0.4em\relax Harlow, England: Addison-Wesley, 1999.

% \end{thebibliography}
\bibliographystyle{IEEEtran}
\bibliography{IEEEabrv,myBib.bib}

% that's all folks
\end{document}
